# Supplementary material for: Representational aspects of depth and conditioning in normalizing flows
Source: arXiv:2010.01155 source file (2021-06-25)
Supplement: Supplementary file 1 [file appendix.tex]

\newpage
\appendix
\section{Appendix}
